# Supplementary material for: Extended Addressing Machines for PCF, with Explicit Substitutions
Source: arXiv:2212.11147 source file (2023-02-20)
Supplement: Supplementary file 1 [file tempappendix.tex]

\begin{proof}[Proof of lemma~\ref{lem:typing}.\ref{lem:typing4}]
Given an \EPCF{} term $M$, an \EPCF{} value $V$, an explicit substitution $\sigma$, a type $\alpha$, and a context $\Gamma$ such that $\substseq{\sigma}M \reddd V, \sigma \models \Gamma, \Gamma \vdash M : \alpha$, we prove by induction on a derivation of $\substseq{\sigma}M \reddd V$ that $\vdash V : \alpha$.

\begin{description}
\item [Case $\valrule$:] In this case $M = V = \num n, \num n \in \nat$, and $\alpha = \tint$. By the typing rules of \EPCF{}, $\vdash \num n : \tint$.

\item [Case $\funrule$:] In this case $M = \lam x.\esubst{M'}{\rho}, V = \lam x.\esubst{M'}{\sigma + \rho}, \alpha = \beta\rightarrow\gamma$. As $\Gamma \vdash \lam x.\esubst{M'}{\rho} : \beta\rightarrow\gamma$, $\exists! \Delta$ such that $\rho \models \Delta, \Gamma, \Delta, x:\beta \vdash M' : \gamma$. As $\sigma \models \Gamma$ and $\rho \models \Delta$, $\sigma + \rho \models \Gamma, \Delta$. Thus by the typing rules of \EPCF{}, $\vdash \lam x.\esubst{M'}{\sigma + \rho} : \beta\rightarrow\gamma$.

\item [Case $\varrule$:] In this case $M = x, \sigma(x) = (\rho, N), \Gamma = \Gamma', x:\alpha$. By the operational semantics of \EPCF{}, $\substseq{\rho}{N}\reddd V$, and by the type system of \EPCF{} as $\sigma \models \Gamma', x:\alpha$, $[x\leftarrow (\rho, N)] \models x: \alpha$ and thus $\rho \models \Delta, \Delta \vdash N : \alpha$. By IH, $\vdash V : \alpha$.

\item [Case $\betarule$:] In this case $M = N \cdot L$. By the operational semantics of \EPCF{}, $\substseq{\sigma}{N}\reddd \lam x.\esubst{N'}{\rho}$ and $\substseq{\rho + [x \leftarrow (\sigma, L)]}{N'} \reddd V$. By the type system of \EPCF{}, $\Gamma \vdash N : \beta\rightarrow\alpha$, $\Gamma \vdash L : \beta$. By IH, $\vdash \lam x.\esubst{N'}{\rho} : \beta\rightarrow\alpha$, and then by the type system of \EPCF{} $\rho \models \Delta, \Delta, x:\beta \vdash N' : \alpha$. By the type system we also have $[x\leftarrow(\sigma, L)]\models x:\beta$, so $\rho + [x\leftarrow(\sigma, L)]\models\Delta,x:\beta$, and thus by IH $\vdash V:\alpha$.
\end{description}
All other cases derive straightforwardly from applying the type system and the induction hypothesis.

\end{proof}
